# Supplementary material for: Ground and excited energy levels can be extracted exactly from a single ensemble density-functional theory calculation
Source: arXiv:1812.02461 source file (2019-02-13)
Supplement: Supplementary file 1 [file supp_mat.pdf]

# Ground and excited energy levels can be extracted exactly from a single ensemble density-functional theory calculation: supplementary material

Killian Deur[1] and Emmanuel Fromager[1]

[1]*Laboratoire de Chimie Quantique, Institut de Chimie, CNRS/Université de Strasbourg, 4 rue Blaise Pascal, 67000 Strasbourg, France*

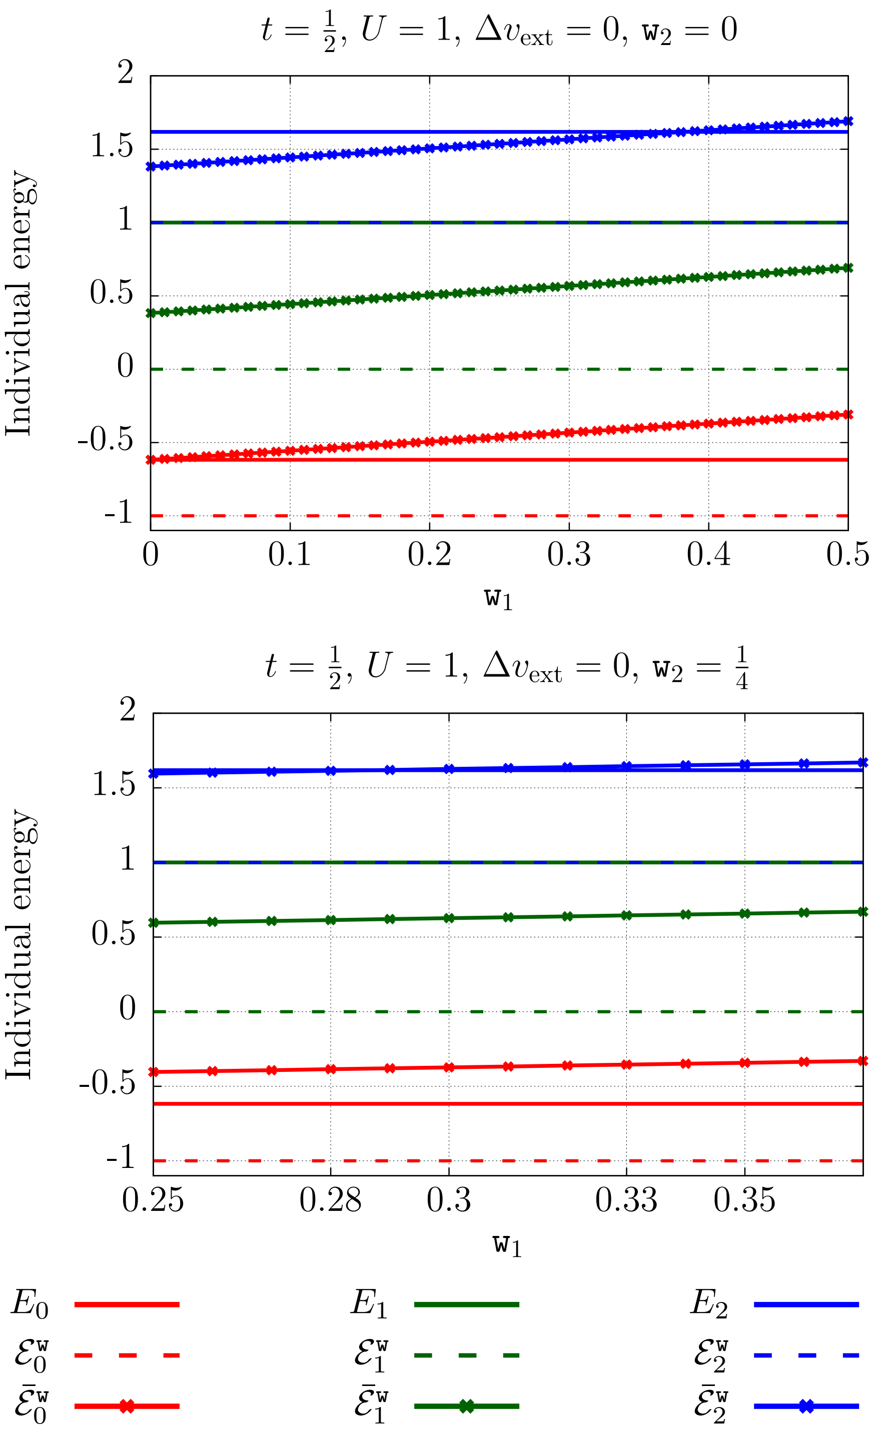


FIG. .1: Unshifted $\mathcal{E}^{\mathbf{w}}_{K=0,1,2}$ and LZ-shifted $\overline{\mathcal{E}}^{\mathbf{w}}_{K=0,1,2}$ KS energies obtained for the symmetric Hubbard dimer (with $U/t = 2$) by varying the first ensemble weight while fixing the second one either to zero (top panel) or 1/4 (bottom panel). Comparison is made with the exact energies $E_{K=0,1,2}$. See text for further details.

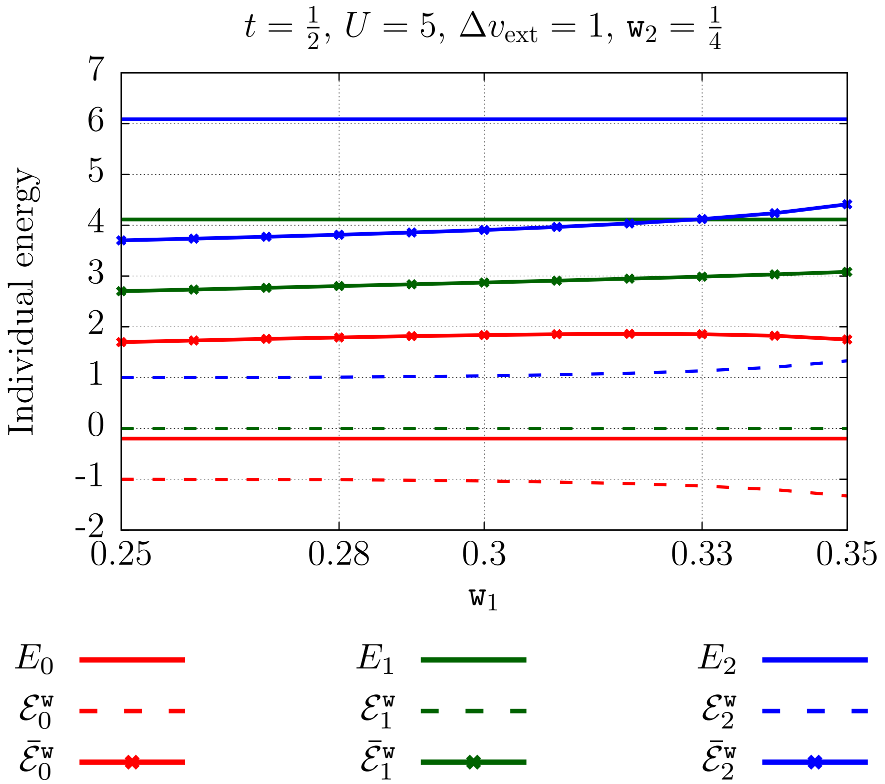


FIG. .2: Same as the bottom panel of Fig. .1 for the asymmetric dimer ($\Delta v_{\text{ext}}/t = 2$) and $U/t = 10$.

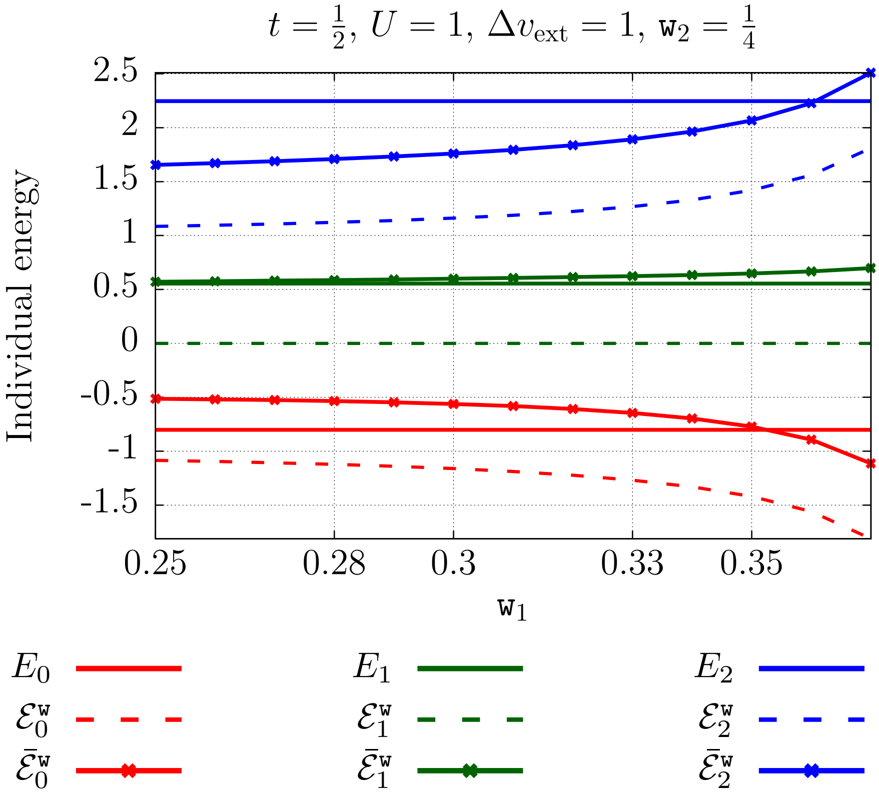


FIG. .3: Same as Fig. .2 with $U/t = 2$.
